# Supplementary material for: Penetrating Shields: A Systematic Analysis of Memory Corruption Mitigations in the Spectre Era
Source: arXiv:2309.04119 source file (2023-09-08)
Supplement: Supplementary file 1 [file appendix.tex]

\appendix
%\section{Tamperproof metadata defense proposals which maintain partial information}
\section{Partial Information}
\label{appendix:partial}

\textbf{Tamperproof metadata defense schemes which maintain partial information} augment a subset of memory accesses with lightweight metadata, providing much more ideal performance compared to defenses maintaining full information. Unlike mitigations which maintain full information, defenses which maintain partial information are diverse in their security goals, and as such, there exists a large variety in defining, maintaining and utilizing metadata. 

For example, Intel CET~\cite{intelcet} Indirect Branch Tracking (IBT) uses \texttt{endbranch} instructions as its metadata. IBT of Intel CET marks valid branch target locations with an \texttt{endbranch} instruction, and the instruction after a branch is checked in the hardware to confirm that it is an \texttt{endbranch} instruction. 
Shadow Stack (SS) of Intel CET leverages the return addresses as its metadata. Intel CET-SS maintains a second stack in a shadow region of the memory that pushes the return addresses to the shadow stack on \texttt{call}s  and pops the return addresses off the shadow stack on \texttt{ret}s. 
ZERO~\cite{zero}, REST~\cite{rest}, and Califorms~\cite{califorms} utilize tagged memory to track their metadata. 
ZERO~\cite{zero} implicitly tags each memory address in the microarchitecture with 2 bits, to mark an address among four different types: data, return adress, data pointer, and function pointer. ZERO enforces pointer integrity by blocking addresses of different types from overwriting another. 
REST~\cite{rest} and Califorms~\cite{califorms} implicitly tags each memory address in the microarchitecture to blacklist memory addresses surrounding allocated objects. By doing so, REST and Califorms provides spatial safety against adjacent buffer overflows.

These defense proposals which leverage only partial information, are also able to cheaply enforce the integrity of their metadata. Intel CET-IBT blocks adversaries from forging rogue \texttt{endbranch} instructions by enforcing W $\oplus$ X to code pages. Intel CET-SS protects the integrity of the shadow stack by extending page table protection with additional attributes. ZERO, REST, and Califorms metadata cannot be modified as the tags are managed implicitly by the micro-architecture.

Despite the tamperproof property, as well as the low overhead of these defenses, the defenses leveraging partial information provide weaker security coverage compared to mitigations leveraging full information.
SS of Intel CET is able to mitigate ROP attacks, but lacks any protection against JOP attacks. 
IBT of Intel CET narrows the attack vector of ROP and JOP attacks by limiting the branch target locations, but does fully mitigate these attacks and can broken by advanced block-oriented programming~\cite{ispoglou2018block}.
ZERO provides pointer integrity, but is vulnerable to data corruption attacks. 
REST is able to protect against adjacent buffer overflows, but provides no protection against non-adjacent buffer overflows. 
Califorms provides protection against non-adjacent buffer overflows, by randomizing the size of the security bytes (i.e., blacklisted addresses), but we find that Califorms is vulnerable to synergistic attacks for non-adjacent buffer overflows (\cref{attackvector}).
